# Supplementary material for: Rapid Risk Minimization with Bayesian Models Through Deep Learning Approximation
Source: arXiv:2103.15682 source file (2021-05-05)
Supplement: Supplementary file 1 [file appendix.tex]

\section{Appendix A}
\glsresetall
In the following appendix, we will first elaborate on some of the hyperparameters used for our experiments. This will be followed by a definition of the Smooth L1-loss \cite{ren2015faster}. Finally, we will conclude with a detailed analysis of our data sampling process' impact on the \gls{nn}'s inference on the invariants present in the domains used throughout the paper.

\subsection{Hyperparameters}
For the Simple \gls{bm} experiment, we set $\widehat{\alpha_1} = 40$, $\widehat{\alpha_2} = 4$, $\widehat{\beta_1} = 0.9$, $\widehat{\beta_2} = 0.5$, and $\widehat{\sigma} = 0.5$, and the priors: $\alpha \sim \mathcal{N}\left(\mu = \left(15,15\right)^T, \sigma = \mathcal{\mathbf{I}}_215\right)$, $\mathbf{\beta} \sim \mathcal{N}\left(\mu = \left(1,1\right)^T, \sigma = \mathcal{\mathbf{I}}_2\right)$, and $\sigma \sim \text{Gamma}\left(1,1\right)$. We used Early Stopping \cite{bishop2006pattern, goodfellow2016deep, Prechelt1998, zhang2016understanding} with a patience of $20$ when fitting all \glspl{nn}. With no improvement of the Smooth L1-loss on the validation dataset for $20$ epochs, we restored the state of the \gls{nn} at to state at the last epoch at which this loss improved, and terminated training. The \gls{al} experiment also applied Early Stopping with a patience of $10$. To measure improvement over \gls{al} iterations, we compared the validation loss across fitted \glspl{nn}.

\subsection{Smooth L1-loss}
For all experiments, we used loss function \emph{Smooth L1-loss} \cite{ren2015faster} for fitting the \glspl{nn} with a learning rate of $1.0 \times 10^{-4}$. The Smooth L1-Loss is defined as: 
\begin{align*}
	\text{Smooth}_{\text{L1}}\left(\mathbf{y}, \widehat{\mathbf{y}} \right) &= \frac{1}{M} \sum_{m \in M} z_m \\
	z_m &= \begin{cases}
		0.5 (\mathbf{y}_m - \widehat{\mathbf{y}}_m)^2, & \text{if } |\mathbf{y}_m - \widehat{\mathbf{y}}_m | < 1 \\
		|\mathbf{y}_m - \widehat{\mathbf{y}}_m| - 0.5, & \text{otherwise}
	\end{cases} 
\end{align*}

Other loss functions could have been used instead, but we found this function to work well in our experiments.

\subsection{Minimizing Risk} 
Assume we can obtain pairs of data samples, $\left(x, y\right)$, from some, unknown, joint probability distribution, $p\left(X, Y\right)$. Now, we are given an observation of the predictor, $x$, and intend to predict the correct corresponding, $y$. We will denote this prediction, $\tilde{y}$.
Basic decision theory establish how one makes the best prediction in such a case. First, we need to quantify how `wrong' any prediction is with respect to the correct prediction. Throughout this paper, we are interested in regression problems and will assume a euclidean loss function. Let $\mathcal{L}\left(\tilde{y}, y\right) = \left(\tilde{y} - y \right)^2$. Our goal is to choose $\tilde{y}$ as to minimize the expected loss, hence $\argmax_{\tilde{y}} \mathbb{E}\left[\mathcal{L}\left(\tilde{y}, y \right) \right]$. This expectation is simply a weighted average over all the possible values for $Y$ multiplied with the conditional probability of that value for $Y$:
\begin{equation}
	\begin{split}
		\mathbb{E}\left[\mathcal{L}\left(\tilde{y}, Y \right) \arrowvert X = x \right] &= \int \mathcal{L}\left(\tilde{y}, y \right) p\left(y \arrowvert X=x \right) \, dy \\
		&= \int \left(\tilde{y} - y \right)^2 p\left(y \arrowvert X=x \right) \, dy \\
	\end{split}
\end{equation}
As we are interested in knowing what the optimal value of $\tilde{y}$ is, we take the partial derivative of $\tilde{y}$. This will inform us how our prediction affects our expected loss:

\begin{equation}
	\begin{split}
		\frac{\partial \mathbb{E}\left[\mathcal{L}\left(\tilde{y}, y \right) \arrowvert X=x \right]}{\partial \tilde{y}} &= 2 \int \left(\tilde{y} - y \right)p\left(y \arrowvert X=x \right) \, dy \\
		&= 2 \left( \tilde{y} - \int y p\left(y \arrowvert X=x \right) \, dy \right) \\
		&= 2 \left( \tilde{y} - \mathbb{E}\left[Y \arrowvert X=x \right] \right)
	\end{split}
\end{equation} 

As we aim to minimize the loss, we set the partial derivative to 0, and solve for $\tilde{y}$
\begin{equation}
	\begin{split}
		2 \left( \tilde{y} - \mathbb{E}\left[Y \arrowvert X=x \right] \right) &= 0 \\
		2 \tilde{y} - 2\mathbb{E}\left[Y \arrowvert X=x \right] &= 0 \\
		2 \tilde{y} &= 2\mathbb{E}\left[Y \arrowvert X=x \right] \\
		\tilde{y} &= \mathbb{E}\left[Y \arrowvert X=x \right] \\
	\end{split}
\end{equation}

Hence the optimal prediction is the conditional expectation of the underlying data distribution. As the ground true data distribution for most interesting problems is unknown, we cannot compute it directly. Instead, one can create a model of it. Although the model will, as any other model, be wrong, it can prove useful for predictions. If we assume a \gls{bm} with a posterior distribution $\phi \sim p\left(\phi \arrowvert \mathcal{D} \right)$, we can use $\mathbb{E}\left[\tilde{Y} \arrowvert X \right]$ as a surrogate for the ground true expected conditional:
\begin{equation}
	\label{eq:posterior_prediction}
	\mathbb{E}\left[\tilde{Y} \arrowvert X \right] = \int \tilde{y} p\left(\tilde{y} \arrowvert X=x \right) d\tilde{y}
\end{equation}
As we are working with a \gls{bm}, the distribution $p\left(\tilde{Y} \arrowvert X=x \right)$ requires marginalizing out the posterior 
\begin{equation}
	p\left(\tilde{y} \arrowvert X=x \right) = \int p\left(\tilde{y} \arrowvert X=x, \phi \right) p\left(\phi \arrowvert \mathcal{D} \right) d\phi
\end{equation}

As a result, doing risk minimization with a \gls{bm} requires computing a double integral. We use the rules of integration:
\begin{equation}
	\label{eq:expectation_given_x_phi}
	\begin{split}
		\mathbb{E}\left[\tilde{Y} \arrowvert X \right] &= \int \tilde{y} \int  p\left(\tilde{y} \arrowvert X=x, \phi \right) p\left(\phi \arrowvert \mathcal{D} \right) \, d\phi \, d\tilde{y}	 \\
		&= \int \int \tilde{y} p\left(\tilde{y} \arrowvert X=x, \phi \right) p\left(\phi \arrowvert \mathcal{D} \right) \, d\phi \, d\tilde{y}	\\
		&= \int \int \tilde{y} p\left(\tilde{y} \arrowvert X=x, \phi \right) p\left(\phi \arrowvert \mathcal{D} \right) d\tilde{y} \, d\phi \\
		&= 	\int \int \tilde{y} p\left(\tilde{y} \arrowvert X=x, \phi \right)  d\tilde{y} p\left(\phi \arrowvert \mathcal{D}\right) \, d\phi \\
		&= 	\int \mathbb{E}\left[ \tilde{Y} \arrowvert X, \phi \right] p\left(\phi \arrowvert \mathcal{D}\right) \, d\phi
	\end{split}
\end{equation}
Integrating out the posterior in the outer integral is in most cases computationally intractable. In such a case, one can apply a 	\gls{mc} simulation \cite{Kroese2014WhyTM, kruger2016predictive}:

\begin{equation}
	\label{eq:mc_sim}
	\begin{split}
		\phi &= \left\{ \phi_m \sim p\left( \phi \, \arrowvert \, \mathcal{D} \right) \right. \\
		\tilde{Y} &= \frac{1}{M} \sum_{m \in M} \mathbb{E}\left[ \tilde{Y} \arrowvert \phi_m, x \right]\\
	\end{split}
\end{equation}

Equation~\eqref{eq:mc_sim} can be run in parallel across CPU cores as each simulation runs independently of the other. Despite \gls{mc} simulation being a simple, efficient, and fairly accurate, approximation, the degree of parallelism is limited to the number of CPU cores available, and consequently insufficient in time-sensitive domains with the need for a high level of accuracy, i.e.\ more posterior samples used for prediction. 

The inner expectation, $\mathbb{E}\left[\tilde{Y} \arrowvert x, \phi_m\right]$, has for most \glspl{bm} a closed form solution which can be computed analytically. One simply needs to perform the sequence of computations step by step in the BM using $x$, $\phi_m$, and the expectation of the involved distributions, e.g. gaussian, poisson, exponential. For the most, simple, \glspl{bm}, this is not a computational burden, and involves only simple, fast, matrix operations. However, for large, complex, hierarchical models, even this property is computationally heavy. As the complexity of the model increases, so does the cost of making predictions --- especially when the computations cannot be done solely through matrix multiplication, but requires loops or multiple, sequential, statements. 

In our paper, we present a method for training a \gls{nn} to predict the inner expectation over a range of pre-generated posterior samples. This allows for computing the expectation using the NN as a surrogate, and provides the full posterior predictive distribution in a single feed-forward pass. The mean of this set of conditional expectations constitutes an \gls{mc} simulation of Equation~\eqref{eq:posterior_prediction}, and can be used for minimizing risk when doing prediction.

\subsection{Learning invariant properties of the domains}

As mentioned in the main text, one of the major challenges in the selected domains is to learn the invariant properties correctly. In this work, the \gls{bm} has the advantage that the creator of the model can explicitly define these invariates and covariates between predictors. If there is a covariation between predictors, the creator of the model can make the objective of the \gls{bm} to find the posterior distribution for the parameters of a covariance matrix with priors the creator finds reasonable.
This is more difficult in the world of \glspl{nn}. There are three popular approaches to learn invariant properties for \glspl{nn}, 1) Tangent propagation \cite{bishop2006pattern} which involves careful modifications to the loss function. 2) The use of weight sharing, one popular application of weight sharing is the use of convolutional layers, and has proven to work well on natural language processing \cite{10.1145/1390156.1390177}, image classification \cite{krizhevsky2012imagenet}, and timeseries data \cite{8010701} as they are space invariant \cite{zhang1988shift}. 3) Modifications to the dataset, e.g. through image rotation and transformation \cite{7560644, zhang2019image, 7797091}. In this paper, we took the approach of learning invariants through the datasampling process. For the domains introduced in this paper, the effect of $\mathbf{x}_j$ on $\mathbf{y}$ is invariant to $\mathbf{x}_{\neq j}$. Inferring this invariance is particularly challenging for predictors having a low effect on $\mathbf{y}$. From the datasampling procedure as presented in \eqref{eq:simple_bm_data_sampling}, we argue how the use of setting $\mathbf{X}_{ij} = 0$ with probability $\text{Bern}\left(1-\tau\right)$ helps learning these invariants. To show $\tau$'s effect on the fitted \gls{nn}, we choose some predictor, $j$, from the `Complex BM' domain. The chosen predictor has a low effect on $\mathbf{y}$, making it hard for the \gls{nn} to single out. To determine the \gls{nn}'s performance on the invariants present in the domain with respect to predictor $j$, we perform two experiments. We will refer to these as 1) \emph{marginalized} experiment and 2) \emph{fixed} experiment. As we are generally interested in the relative \emph{effect} $\mathbf{x}_j$ has on $\mathbf{y}$, we let $g\prime \left( \mathbf{x} \right) = g\left( \mathbf{x}\right) - g\left(\mathbf{x}^{\prime} \right)$ where $\mathbf{x}^{\prime} = \mathbf{x}$ except for $\mathbf{x}^{\prime}_j = 0$. For the marginalization approach, we marginalize out all other predictors, $\mathbf{x}_{\neq j}$, as so $y = \int g\prime\left( \mathbf{x} \right) p\left(\mathbf{x}_{\neq j} \right) d\mathbf{x}_{\neq j}$. We let $\mathbf{x}_{\neq j}$ follow a uniform distribution, and use \gls{mc} sampling to approximate the integral. In figure \ref{fig:dropout_margin}, the approach is visualized for increasing values of $\mathbf{x}_j$.
\begin{figure}[b!]
	\centering
	\includegraphics[width=\linewidth]{dropout/paidprint_margin}
	\caption{The marginalized invariance for predictor $j$. The black, dashed, line is the ground true value of $y$. Each line indicates a \gls{nn}'s predictions using $\mathbf{x}$ keeping $\mathbf{x}_j$ fixed and marginalizing out the other predictors. Each \gls{nn} is trained using a different value of $\tau$. We find the optimum value for $\tau$ being either 0.6 or 0.8 in this example.}
	\label{fig:dropout_margin}
\end{figure}
As the \gls{nn} takes a \gls{ohe} for the day of week as input, we have chosen a single, random, day for these experiments. The figure shows the result of the marginalization procedure for five distinct \glspl{nn}. The only difference between the \glspl{nn} is the $\tau$ used for generating the training dataset of 100,000 examples. From the figure it is clear that disabling the `dropout' completely, i.e. $\tau = 1$, performs worse compared to $\tau = 0.6$ and $\tau = 0.8$. Likewise, setting $\tau$ too low yields an inefficient datasampling process, as most values of $\mathbf{X}_{IJ}$ are 0 and a larger training dataset is needed for a proper fit. The black, dashed, line is the ground true values of $\mathbf{y}$ generated using the \gls{bm}. The shaded area constitutes the 95\% confidence interval for the value of $y$. This confidence interval is calculated using $\sigma\left(\mathbf{y} \right)$ since $\mathbf{y} = g \left( \mathbf{x} \right)$ is an $M$ dimensional vector, with one prediction for each posterior sample. We used no less than 1000 \gls{mc} samples to measure the NN's marginalized prediction over $y$. Even with the large quantity of samples, the predictions of the NN trained with $\tau = 1$ still oscillate substantially compared to the \glspl{nn} for which $\tau < 1$.

Next, we use the same \glspl{nn} and predictor, $j$, for the \emph{fixed} experiment. Here, we simply set $\mathbf{x}_{\neq j}$ to some constant, $c$, and calculate $g\prime\left( \mathbf{x}\right)$. We perform the procedure for three values of $c$, and the result is shown in figure \ref{fig:fixed invariant experiment}.

\begin{figure*}[tb!]
	\centering
	\begin{subfigure}[b]{0.33\textwidth}
		\centering
		\includegraphics[width=\textwidth]{dropout/paidprint_fixed_0.0.pdf}
	\end{subfigure}
	\hfill
	\begin{subfigure}[b]{0.33\textwidth}
		\centering
		\includegraphics[width=\textwidth]{dropout/paidprint_fixed_0.5.pdf}
	\end{subfigure}
	\hfill
	\begin{subfigure}[b]{0.33\textwidth}
		\centering
		\includegraphics[width=\textwidth]{dropout/paidprint_fixed_1.0.pdf}
	\end{subfigure}
	\caption{The \emph{fixed} experiments for determining the \glspl{nn} inference on the invariants in the domain. We show five trained \glspl{nn} for various values of $\tau$ for predictor $j$ with $\mathbf{x}_{\neq j} = c$ for $c \in \left\{0, 0.5, 1 \right\}$. Predictor $j$ has a relatively weak impact on $y$, making it harder for the \gls{nn} to learn its effect. Across all values of $c$, the \gls{nn} trained with $\tau = 0.8$ yields the best overall performance.}
	\label{fig:fixed invariant experiment}
\end{figure*}

Learning the invariant properties of this domain to perfection would result in three curves being identical across all values for $c$ and all lie on the dashed, black, curve. Performing well on this experiment is generally harder than the marginalized version, as we choose extreme values for $c$ when measuring the \glspl{nn} performance on the invariants. This makes the measure a better indicator of whether the \glspl{nn} has learned the generalized features of the domain. This is a strictly needed requirement for our input optimization experiments, as these tend to push predictors to the extremes depending on the constraint $\mathcal{B}$ from \eqref{eq:loss}. In contrast, for the \gls{nn} to perform well on the marginalized experiment, it simply needs to perform well on average over $N$ uniform samples of predictors $\neq j$.

As can be seen in figure \ref{fig:fixed invariant experiment}, the \gls{nn} trained using $\tau = 0.8$ provides the best performance across various $c$s. For $\tau = 1.0$ and $c = 0$ the \gls{nn} has no perception of the effect $\mathbf{x}_j$ has on $y$. The predictor, $j$, chosen for these experiments, were chosen as it has a low effect on $y$. If we instead choose another predictor, $j\prime$, with a significantly higher impact on $y$, setting $0.5 \leq \tau < 1$ still yields better results, but the difference is reduced. This is shown in figure \ref{fig:fixed invariant experiment_j_mark} and \ref{fig:dropout_margin_j_mark}.
\begin{figure*}[htb!]
	\centering
	\begin{subfigure}[b]{0.33\textwidth}
		\centering
		\includegraphics[width=\textwidth]{dropout/paiddigitaldisplay_fixed_0.0.pdf}
	\end{subfigure}
	\hfill
	\begin{subfigure}[b]{0.33\textwidth}
		\centering
		\includegraphics[width=\textwidth]{dropout/paiddigitaldisplay_fixed_0.5.pdf}
	\end{subfigure}
	\hfill
	\begin{subfigure}[b]{0.33\textwidth}
		\centering
		\includegraphics[width=\textwidth]{dropout/paiddigitaldisplay_fixed_1.0.pdf}
	\end{subfigure}
	\caption{The \emph{fixed} experiments for determining the \glspl{nn} inference on the invariants in the domain. We show five trained \glspl{nn} for various values of $\tau$ for predictor $j\prime$ with $\mathbf{x}_{\neq j\prime} = c$ for $c \in \left\{0, 0.5, 1 \right\}$. $j\prime$ has a high impact on $y$, making the signal to be learned by the \gls{nn} stronger, hence an easier task. Across all values of $c$, the \gls{nn} trained with $\tau = 0.8$ yields the best overall performance.}
	\label{fig:fixed invariant experiment_j_mark}
\end{figure*}
\begin{figure}[tb]
	\centering
	\includegraphics[width=\linewidth]{dropout/paiddigitaldisplay_margin}
	\caption{The marginalized invariance for the predictor $j\prime$ with a stronger effect on $y$. All \glspl{nn} acknowledge $j\prime$'s effect on $y$, with $\tau = 0.8$ producing the best fit, and $\tau = 1.0$ still fluctuating considerably compared to the NN for which $\tau < 1$.}
	\label{fig:dropout_margin_j_mark}
\end{figure}
On the $y$-axis of the figures, one can see the higher impact $\mathbf{x}_{j\prime}$ has on $y$ compared to $\mathbf{x}_j$ from figure \ref{fig:dropout_margin} and \ref{fig:fixed invariant experiment}. The increased effect $\mathbf{x}_{j\prime}$ has on $y$ makes it easier for the \gls{nn} to learn this particular invariant.

Using this approach and setting $0.6 \leq \tau < 1$, the invariant properties of the domain are better approximated by the \gls{nn}. The difference between the fitted \glspl{nn} across values for $\tau$ diminishes as the size of the dataset goes towards infinity. However, for the domains examined in this paper, generating the training dataset is a computationally heavy task, as it requires taking $\mathbb{E}\left[y \arrowvert \mathbf{X}_{i*}, \phi_m  \right]$ for each example $i \in I$, and each posterior sample, $m \in M$ using the computationally heavy \gls{bm}. Thus keeping the size of the training dataset at a minimum is required. 

One could potentially learn the \gls{nn} the same invariants through another data sampling process, e.g. by sampling $c \sim p\left(C\right)$ and sample $N$ instances of $\left[\mathbf{X}_{n,\neq j} \sim p\left(X\right)\right]_{n=1}^N$ with $\left[\mathbf{X}_{nj} = c\right]_{n=1}^N$. By keeping some predictor, $j$, fixed, and sample $N$ examples varying all other predictors is similar to image rotation commonly used for training \gls{cnn} classifiers \cite{7560644, zhang2019image, 7797091}, except the corresponding $y$ would change in our domain, which usually is not the case with image rotation and \gls{cnn} classifiers. 
\clearpage
\bibliography{references}

%\todo{Experiment with NN architecture?}
%\todo{Plot model complexity vs eval time}
%\todo{Create fig 6 plot for toy problem and rosenbrock?}
